# Supplementary material for: Domain walls in topological phases and the Brauer-Picard ring for $\operatorname{Vec}(\mathbb{Z}/p\mathbb{Z})$
Source: arXiv:1806.01279 source file (2018-10-25)

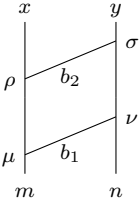

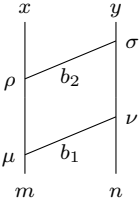

Supplement: Supplementary file 2 [file Appendix_Ladder2.pdf]
